# Supplementary material for: D$^2$USt3R: Enhancing 3D Reconstruction for Dynamic Scenes
Source: arXiv:2504.06264 source file (2025-10-31)
Supplement: Supplementary file 1 [file 4_limitation.tex]

\section*{C. Limitation}
% Optical flow pseudo GT limitation.
